# Supplementary material for: IFC-SSL-Bench: Benchmarking Self-Supervised Learning for Annotation-Efficient Multispectral Imaging Flow Cytometry
Source: arXiv:2610.31848 source file (2026-10-22)
Supplement: Supplementary file 2 [file 04_Article_SupplementaryTables.tex]

%  CONFIGURE NEW SINGLE-PAGE FORMAT 

\onecolumn % go back to one column
\fancyhead{} % make sure we get no headers
\renewcommand{\floatpagefraction}{0.1}
\lfoot[\bSupInf]{\dAuthor}
\rfoot[\dAuthor]{\cSupInf}
\newpage

\captionsetup*{format=largeformat} % make legend slightly larger than in the paper
\setcounter{table}{0} % reset table counter for Supplementary Video Figures
%\setcounter{page}{1} % reset page count
\makeatletter 
\renewcommand{\thetable}{S\@arabic\c@table} % make Table legend start with Table S
\makeatother

%  MAIN TEXT 
\newpage
\section*{Supplementary Tables}

\bigskip

\begin{table}[!h]
    \centering
    \small
    \begin{tabular}{p{3cm}|p{2.2cm} p{2.2cm} p{2.2cm} p{2.2cm} p{2.2cm}}
        Movie & US Release Date & Director & Screenwriter(s) & Story by & Producer\\
        \hline
        Episode IV – A New Hope & May 25, 1977 & \multicolumn{3}{c}{George Lucas} & Gary Kurtz\\
        Episode V – The Empire Strikes Back & May 21, 1980 & Irvin Kershner & Leigh Brackett and Lawrence Kasdan & George Lucas & Gary Kurtz\\
        Episode VI – Return of the Jedi & May 25, 1983 & Richard Marquand & Lawrence Kasdan and George Lucas & George Lucas & Howard Kazanjian\\
    \end{tabular}
    \caption{\textbf{Original ``Star Wars'' Trilogy}\\
    Extracted from \url{https://en.wikipedia.org/wiki/List_of_Star_Wars_films}.}
    \label{supptab:st1}
\end{table}
